# Supplementary material for: Speech Gesture Generation from the Trimodal Context of Text, Audio, and Speaker Identity
Source: arXiv:2009.02119 source file (2020-09-04)

(a) Audio encoder

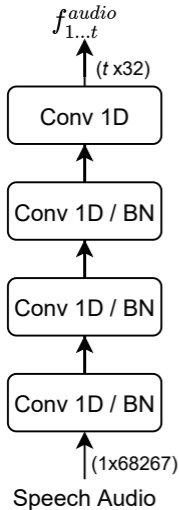

(b) Text encoder

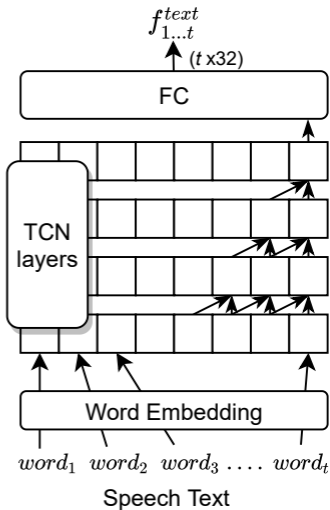

(c) Style embedding

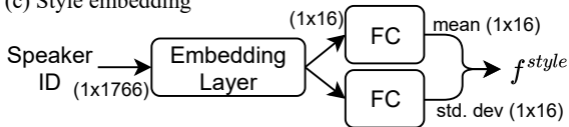

Supplement: Supplementary file 1 [file appendix_encoder.pdf]
