# Supplementary material for: Speech Gesture Generation from the Trimodal Context of Text, Audio, and Speaker Identity
Source: arXiv:2009.02119 source file (2020-09-04)

(a) Gesture generator

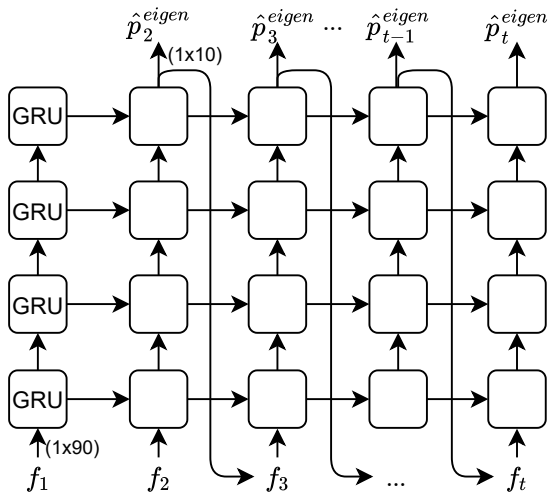

(b) Gesture discriminator

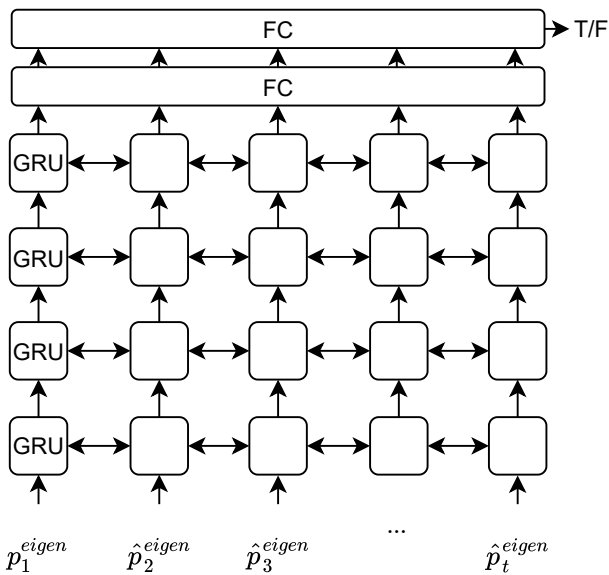

Supplement: Supplementary file 2 [file appendix_generator.pdf]
